# Supplementary material for: GenH2R: Learning Generalizable Human-to-Robot Handover via Scalable Simulation, Demonstration, and Imitation
Source: arXiv:2401.00929 source file (2024-06-14)
Supplement: Supplementary file 2 [file X_suppl.tex]

\clearpage
\setcounter{page}{1}
\maketitlesupplementary
